# Supplementary material for: Planted: a dataset for planted forest identification from multi-satellite time series
Source: arXiv:2406.18554 source file (2024-05-24)
Supplement: Supplementary file 1 [file SI_bs_lr.tex]

\begin{figure}
    \centering
    \includegraphics[width=0.5\linewidth]{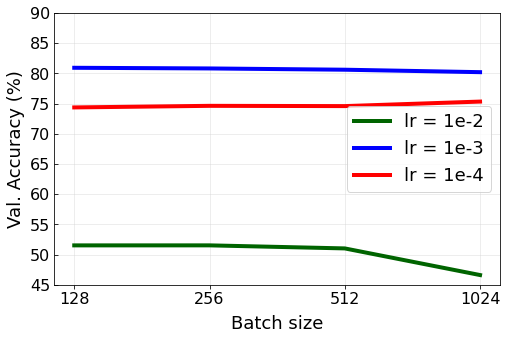}
    \caption{Effect of batch size and learning rate on mean validation accuracy for individual satellites. We did not evaluate on groups of satellites.}
    \label{fig:SI_bs_lr}
\end{figure}
